# Supplementary material for: A Survey on Physarum Polycephalum Intelligent Foraging Behaviour and Bio-Inspired Applications
Source: arXiv:2103.00172 source file (2021-05-08)
Supplement: Supplementary file 1 [file SM_AA.tex]

\begin{equation}
\label{equ:Model/sm_aa}
    P\_AA_{(i,j),(k,l)} =
    \begin{cases}
      1, & \text{if}\ CT_{(k,l)} = "FREE" \\
      1, & \text{if}\ CT_{(k,l)} = "PHYSARUM",\\
         & ~PID_{(i,j)} = PID_{(k,l)} \\
      0, & \text{otherwise}
    \end{cases}
\end{equation}

where
$CT_{(k,l)}$ represents the cell type as defined in Equation \ref{equ:Model/Cell_Type}.\\
$PID_{(i,j)}$ is the ID of the Physarum at cell $c_{(i,j)}$.\\
