# Supplementary material for: A Survey on Physarum Polycephalum Intelligent Foraging Behaviour and Bio-Inspired Applications
Source: arXiv:2103.00172 source file (2021-05-08)
Supplement: Supplementary file 2 [file SM_AttForce.tex]

\begin{equation}
\label{equ:Model/sm_attforce}
\begin{multlined}
P\_AttForce^{t}_{(i,j),(k,l)} = \\
\left \{
  \begin{aligned}
    &WM_{(i,j)} * \dfrac{CM^{t}_{(k,l)}}{Total\_NCM_{(i,j)}} + WQ_{(i,j)} * \dfrac{CQ^{t}_{(k,l)}}{Total\_NCQ_{(i,j)}}, \\
    & \hspace{3cm} \text{if}\ CM^{t}_{(k,l)} = MAX(CM^{t}_{(i,j)})\\
    &0, \hspace{5cm} \text{otherwise}
  \end{aligned} \right.
\end{multlined}
\end{equation}
\begin{equation*}
\begin{multlined}
WM_{(i,j)} = \dfrac{PH^{t}_{(i,j)}}{100},
WQ_{(i,j)} = \dfrac{100 - PH^{t}_{(i,j)}}{100}
\end{multlined}
\end{equation*}

where
$P\_AttForce_{(i,j),(k,l)}$ defines the value of attraction forces applied on Physarum at cell $c_{(i,j)}$ coming from its neighbouring cell $c_{(k,l)}$.\\
$WM_{(i,j)}$ is the weight assigned to the chemical mass that will attract Physarum to it.\\
$CM^{t}_{(k,l)}$ is the current mass of the chemical at iteration $(t)$ for cell $c_{(k,l)}$.\\
$Total\_NCM_{(i,j)}$ is the total summation of chemical mass for the first neighbour of cell $c_{(i,j)}$.\\
$WQ_{(i,j)}$ is the weight assigned to the chemical quality that will attract Physarum to it.\\
$CQ^{t}_{(k,l)}$ is the current quality of chemical at iteration $(t)$ for cell $c_{(k,l)}$, where $CQ \in [0-10]$; 0: Low quality, 10: High quality.\\
$Total\_NCQ_{(i,j)}$ is the total summation of chemical quality for the first neighbour of cell $c_{(i,j)}$.\\
$MAX(CM^{t}_{(i,j)})$ is a function which returns the maximum value of chemical mass among the neighbourhood of cell $c_{(i,j)}$.\\
$PH_{(i,j)}$ is the hunger motivation of the Physarum, where $PH \in [0-100]$; 0:Satiated, 100:Hungry.\\
