# Supplementary material for: A Survey on Physarum Polycephalum Intelligent Foraging Behaviour and Bio-Inspired Applications
Source: arXiv:2103.00172 source file (2021-05-08)
Supplement: Supplementary file 3 [file SM_RepForce.tex]

\begin{equation}
\label{equ:Model/sm_repforce}
\begin{multlined}
P\_RepForce^{t}_{(i,j),(k,l)} = \\
\left \{
  \begin{aligned}
    & \dfrac{PM^{t}_{(2i-k~,~2j-l)}}{Total\_NPM_{(i,j)}} && \text{if}\ PID_{(i,j)} \neq PID_{(2i-k~,~2j-l)},\\
    & && \hspace{0.25cm} PM^{t}_{(2i-k~,~2j-l)} > Rep\_Limit\\
    &0, && \text{otherwise}
  \end{aligned} \right.
\end{multlined}
\end{equation}

where
$P\_RepForce_{(i,j),(k,l)}$ defines the value of repulsion forces applied on Physarum at cell $c_{(i,j)}$ exerted by its neighbouring cell $c_{(k,l)}$.\\
$PM^{t}_{(2i-k~,~2j-l)}$ is the neighbour Physarum mass at the opposite direction of cell $c_{(k,l)}$ with reference to the centre point $c_{(i,j)}$ as defined in Equation \ref{equ:Model/Opp_Dir}.\\
$Total\_NPM_{(i,j)}$ is is the total summation of Physarum mass for the first neighbour of cell $c_{(i,j)}$.\\
$Rep\_Limit$ is a limit where Physarum must reach to repel neighbouring Physarum.\\
