# Supplementary material for: A Survey on Physarum Polycephalum Intelligent Foraging Behaviour and Bio-Inspired Applications
Source: arXiv:2103.00172 source file (2021-05-08)
Supplement: Supplementary file 4 [file SM_Diff.tex]

\begin{equation}
\label{equ:Model/sm_diff}
\begin{multlined}
   PM^{t+1}_{(i,j)} = PM^{t}_{(i,j)} +\\
   \sum_{(k,l)} \left \{
    \begin{aligned}
      & (PF * PD) (PM^{t}_{(k,l)} - PM^{t}_{(i,j)}) \\ 
       & \hspace{3cm}  \text{if}\ P\_AA_{(i,j),(k,l)} = 1, \\
       & \hspace{3cm} PM^{t}_{(i,j)} > Diff\_limit\\
       &0, \hspace{2.7cm} \text{otherwise}
     \end{aligned} \right.
\end{multlined}
\end{equation}
\begin{equation*}
   \begin{aligned}
   &\forall (k,l) : &&i - 1 \leqslant k \leqslant i + 1,\\
   &				   &&j - 1 \leqslant l \leqslant j + 1,\\
    &                &&k \neq l
   \end{aligned}
\end{equation*}
\begin{equation*}
PF = 1 + P\_AttForce_{(i,j),(k,l)} + P\_RepForce_{(i,j),(k,l)}
\end{equation*}

where
$PM^{t+1}_{(i,j)}$ defines the diffusion of Physarum mass for the next generation $(t+1)$ at cell $c_{(i,j)}.$\\
$PM^{t}_{(i,j)}$ is the current mass of Physarum at cell $c_{(i,j)}$.\\
$PM^{t}_{(k,l)}$ is the current mass of neighbouring Physarum at cell $c_{(k,l)}$.\\
$P\_AA^{t}_{(i,j),(k,l)}$ defines whether Physarum at cell $c_{(i,j)}$ is available to diffuse towards a neighbouring cell $c_{(k,l)}$ as defined in Equation \ref{equ:Model/sm_aa}.\\
$PD$ is the Physarum diffusion coefficient.\\
$Diff\_Limit$ is the limit which in which the Physarum mass must exceed in order to diffuse.\\
$PF$ is the sum of forces affecting Physarum.\\
%$P\_AttForce_{(i,j),(k,l)}$ defines the value of attraction forces applied on Physarum at cell $c_{(i,j)}$ coming from its neighbouring cell $c_{(k,l)}$ as defined in Equation \ref{equ:Model/sm_attforce}.\\
%$P\_RepForce_{(i,j),(k,l)}$ defines the value of repulsion forces applied on Physarum at cell $c_{(i,j)}$ exerted by its neighbouring cell $c_{(k,l)}$ as defined in Equation \ref{equ:Model/sm_repforce}.\\
