# Supplementary material for: A Survey on Physarum Polycephalum Intelligent Foraging Behaviour and Bio-Inspired Applications
Source: arXiv:2103.00172 source file (2021-05-08)
Supplement: Supplementary file 5 [file SM_DiffOther.tex]

\begin{equation}
 \label{equ:Model/smdiff}
 \begin{multlined}
  SM^{t+1}_{(i,j)} = SM^{t}_{(i,j)} +\\
  \sum_{(k,l)} \left \{
   \begin{aligned}{}
      &\big(SF * SD * SM^{t}_{(k,l)}\big) - SM^{t}_{(i,j)} \hspace{0.15cm} \\ &\text{if}\ SM\_AA_{(k,l)} = 1,\\ 
&SM^{t}_{(i,j)} > Diff\_limit \hspace{0.10cm}0, \\ 
 &\text{otherwise}
    \end{aligned} \right.
  \\
   \begin{aligned}{}
    &\forall (k,l) : &&i - 1 \leqslant k \leqslant i + 1,\\
   &				   &&j - 1 \leqslant l \leqslant j + 1,\\
    &                &&k \neq l
    \end{aligned}
  \\
  \\
  SF = 1 + SM\_AttForce^{t}_{(i,j),(k,l)} + SM\_RepForce^{t}_{(i,j),(k,l)}
 \end{multlined}
 \end{equation}
